# Supplementary material for: Human-instructed Deep Hierarchical Generative Learning for Automated Urban Planning
Source: arXiv:2212.00904 source file (2022-12-01)
Supplement: Supplementary file 1 [file appendix.tex]

\newpage

\begin{center}
\textbf{\fontfamily{ppl} \fontsize{13}{0}\selectfont
Appendix
}%
\bigskip
\end{center}

In the appendix, we introduce supplementary information of our automated urban planner and make other people understand this work further.

\noindent\textbf{Hyperparameter Settings, and Reproducibility}
The learning process of our framework IHPlanner can be divided into two phases: coarse-grained generation and fine-grained generation.
For the coarse-grained generation part  (section ~\ref{cg_part}),
the generator is composed of three transpose convolution layers and the discriminator is constituted by two convolution layers with a dropout rate of 0.3.
We set the value of $\lambda$ contained in equation ~\ref{loss_g} as 0.8 and employed Adaptive Moment Estimation (Adam) to optimize the model with a learning rate of 0.0001 for 500 epochs.
For the fine-grained generation part  (section ~\ref{fg_part}), 
the feed forward layer is constructed by two linear layers and the planning layers are customized neural network layers.
The two kinds of layers are activated by the relu function.
We utilized 8 heads to extract correlations among urban functionality projections and trained the fine-grained part by an Adam optimizer with a rate of 0.001 for 500 learning epochs.

% \vspace{-0.25cm}
\noindent\textbf{Environmental Settings}
All experiments were conducted using the Ubuntu 18.04.5 LTS operating system, Intel(R) Core(TM) i9-10900X CPU@ 3.70GHz, and 1 way SLI Titan 3090 and 128GB of RAM, with the framework of Python 3.8.5, Tensorflow 2.4.1.

\label{data_distribution}
% \vspace{-0.1cm}
\begin{figure}[!htbp]
\centering
\includegraphics[width=0.8\linewidth]{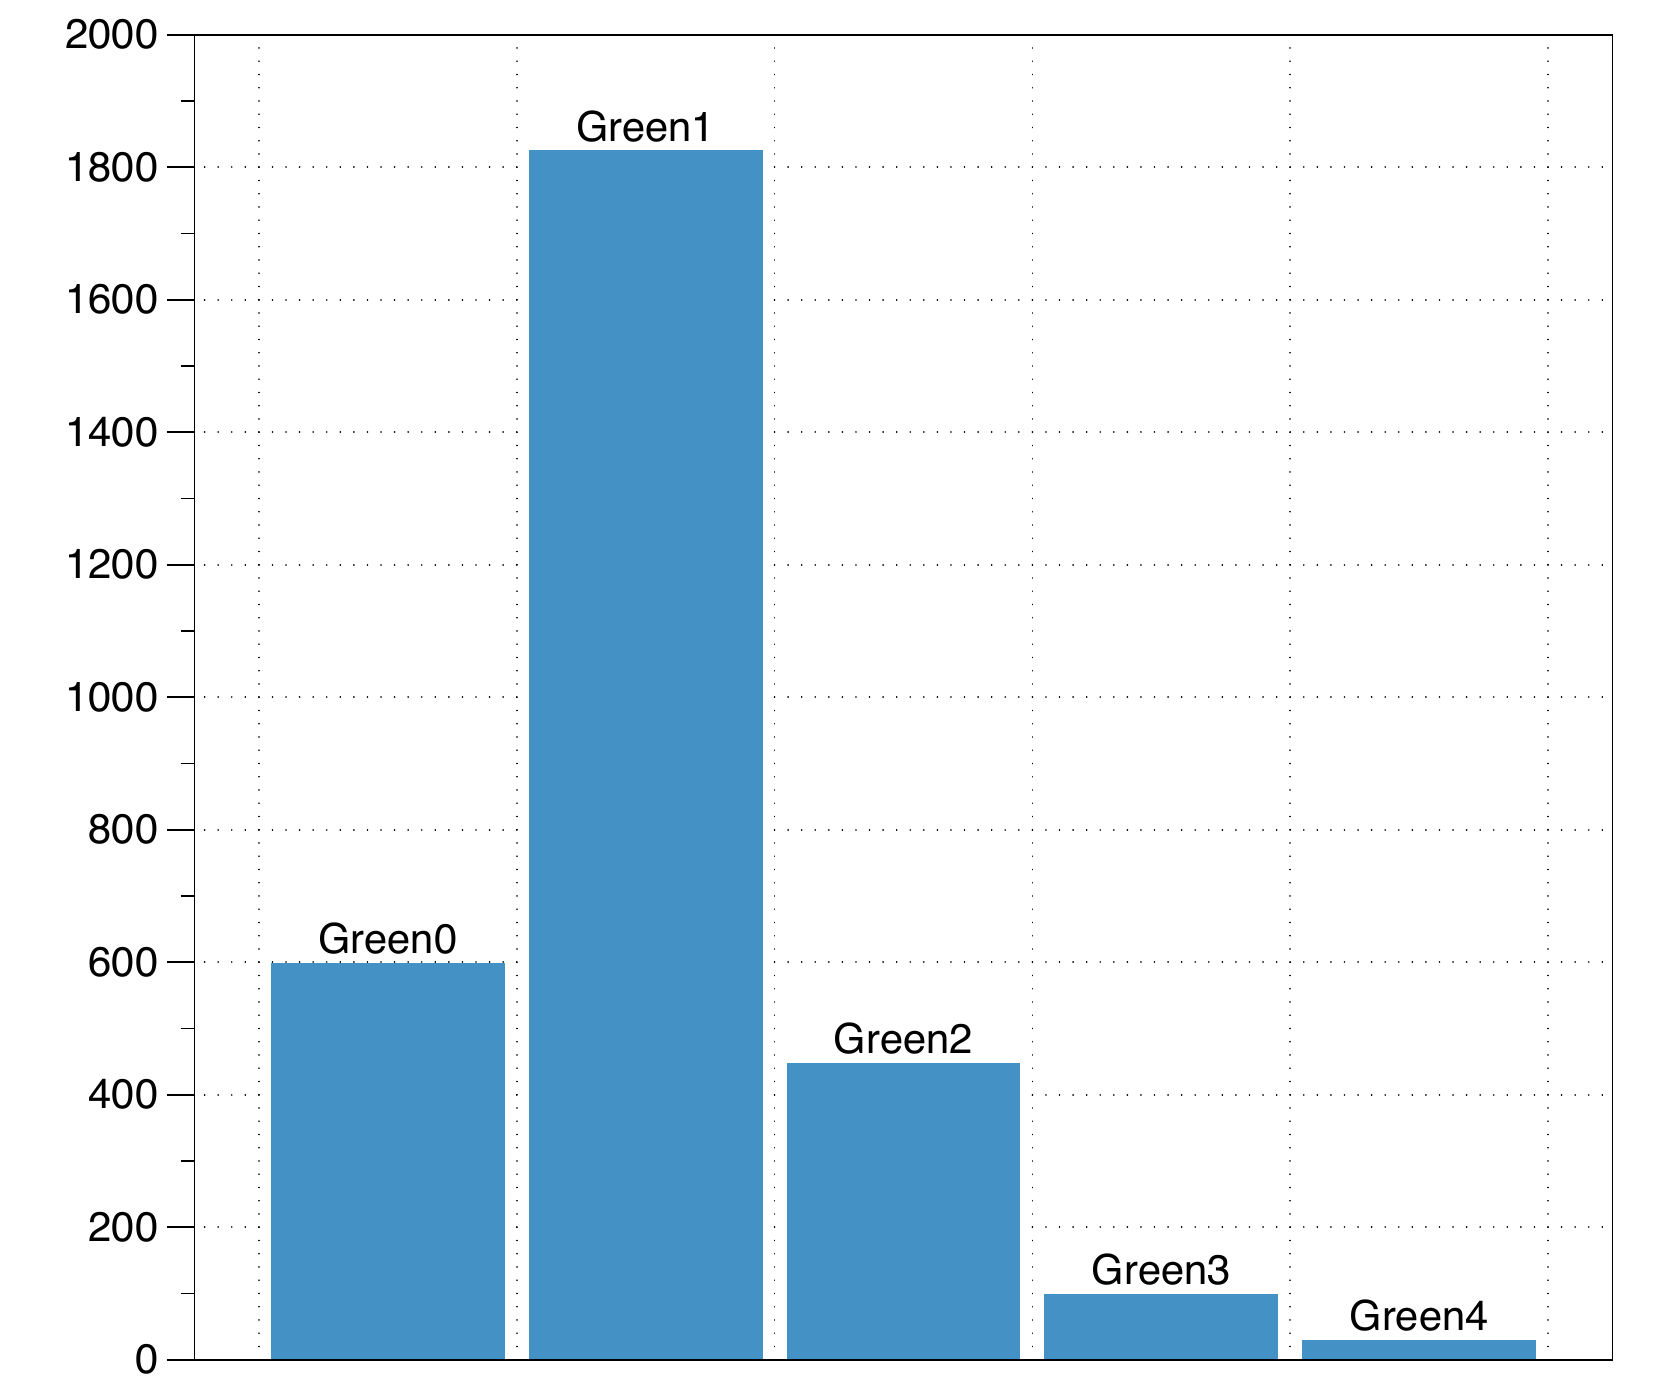}
% \vspace{-0.2cm}
\captionsetup{justification=centering}
% \vspace{-0.2cm}
\caption{Under different green rate levels, the data proportions of configuration samples.}
% \vspace{-0.1cm}
\label{fig:data_dis}
\end{figure}

\noindent \textbf{Data Distribution.}
In our paper, we regarded the green rate level as the human instruction.
There are five kinds of human instructions in our dataset: Green0, Green1, Green2, Green3, Green4.
According these human instructions, the whole dataset is divided into five parts.
The proportion of each part is illustrated in Figure ~\ref{fig:data_dis}.
From this figure, we can find that from the data size perspective, Green1 $>$ Green0 $>$ Green2 $>$ Green3 $>$ Green4.
So, how can we deal with the unbalanced situation during the model generation process is a big challenge. 
In our framework, we adopted the conditioning augmentation module to augment the data diversity, which mitigates the unbalanced question and avoids model overfitting.

% \vspace{-0.3cm}
\begin{figure}[!htbp]
\centering
\includegraphics[width=0.8\linewidth]{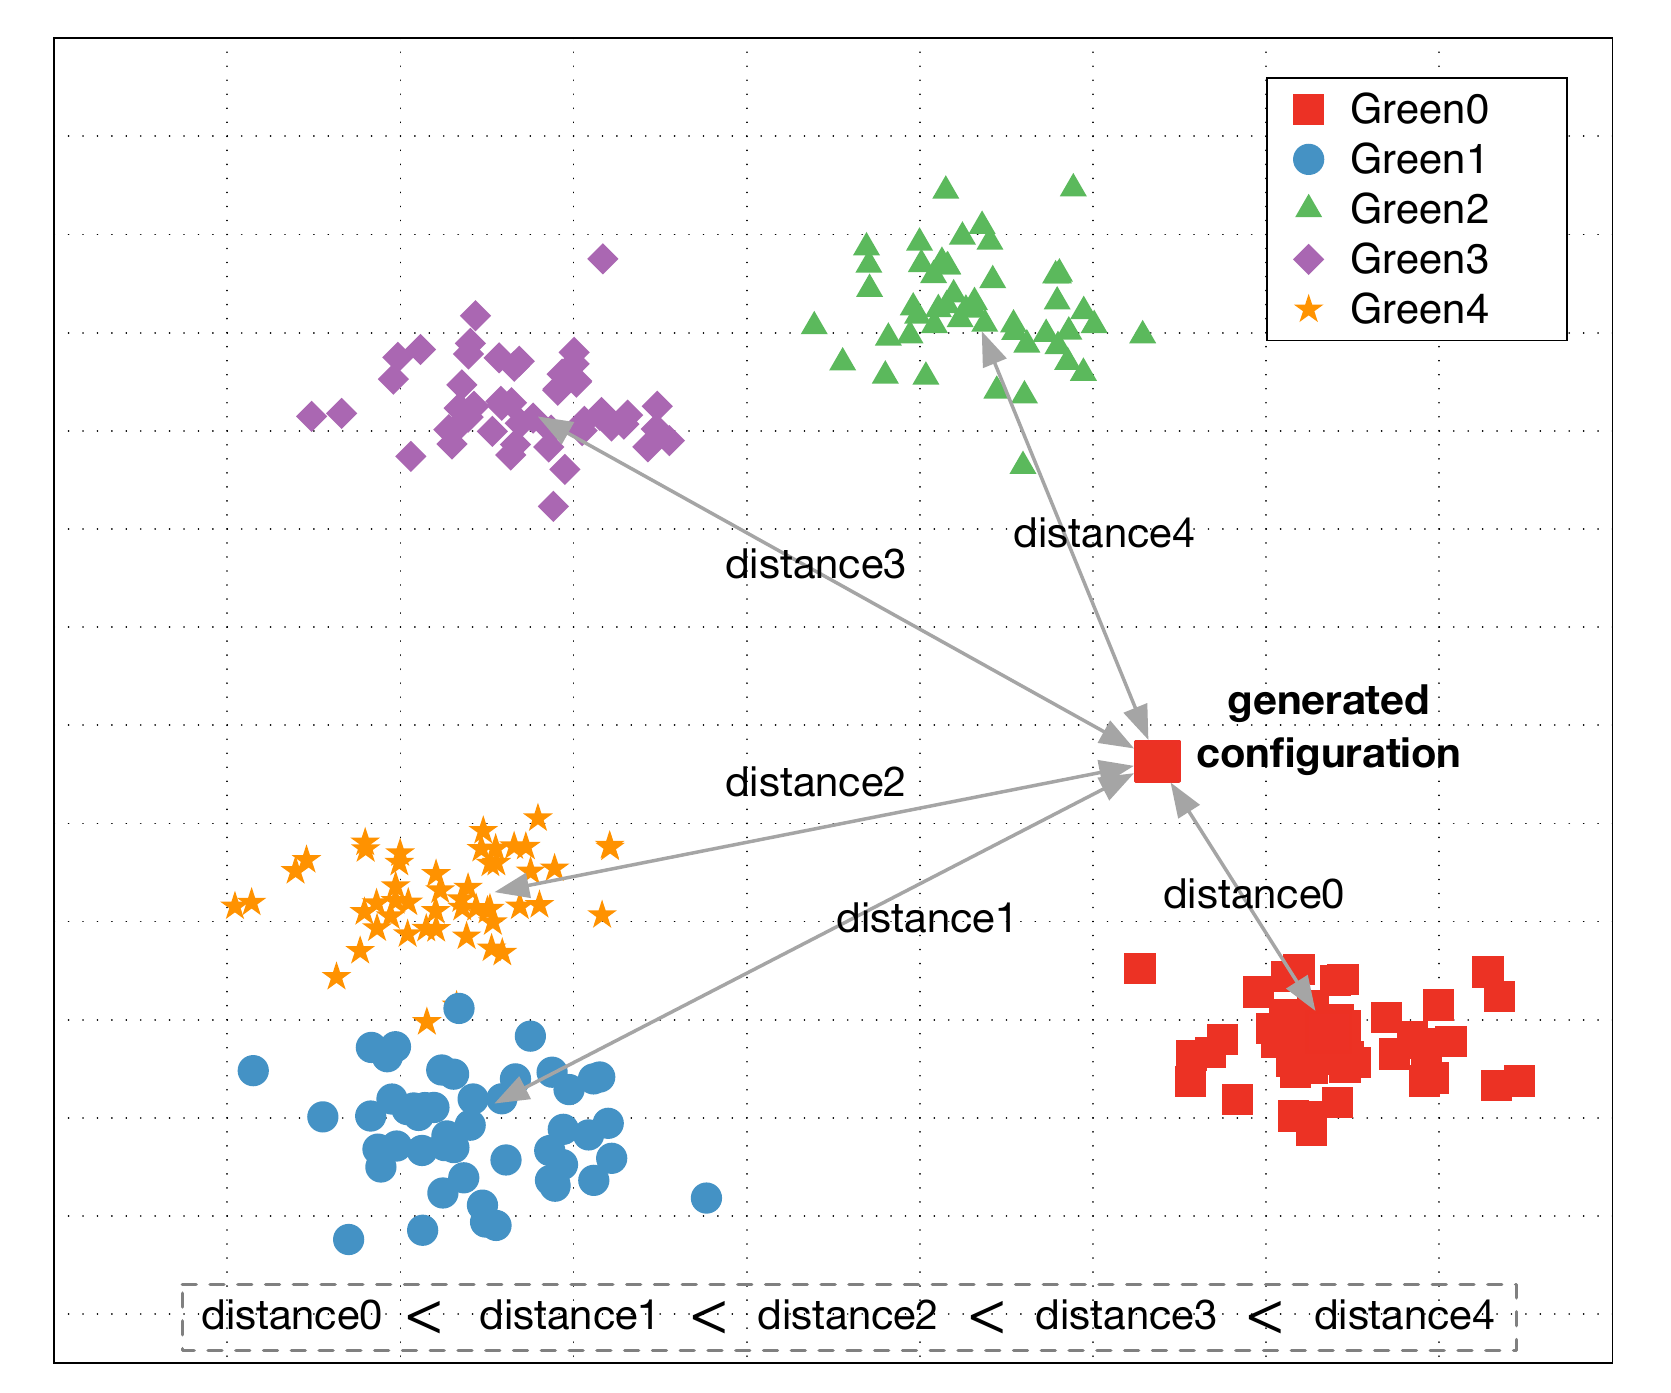}
\vspace{-0.2cm}
\captionsetup{justification=centering}
% \vspace{-0.2cm}
\caption{The distances between the generated configuration and different clusters.}
\vspace{-0.1cm}
\label{fig:reason_evaluate}
\end{figure}

\noindent \textbf{Explanation of Evaluation Metrics}
From the section ~\ref{data_distribution}, we have known that the dataset can be divided into 5 parts according to human instructions.
Thus, as illustrated in Figure \ref{fig:reason_evaluate}, the data distribution is divided into 5 clusters. 
A generated land-use configuration is produced based on a specific human instruction.
In the configuration  space, the distance between the generated configuration and the cluster owning the same label with the human instruction of the configuration should be less compared with the distance between the generated configurations and other clusters.
Thus, we can utilize the distribution divergence to measure the generated performance of all models.
